# Supplementary material for: Variational Optimization of Annealing Schedules
Source: arXiv:1502.05313 source file (2015-03-27)
Supplement: Supplementary file 1 [file supplementary.tex]

%#!pdflatex
%%%%%%%%%%%%%%%%%%%%%%%%%%%%%%%%%%%%%%%%%%%%%%%%%%%%%%%%%%%%%%%%%%
%%%%%%%% ICML 2015 EXAMPLE LATEX SUBMISSION FILE %%%%%%%%%%%%%%%%%
%%%%%%%%%%%%%%%%%%%%%%%%%%%%%%%%%%%%%%%%%%%%%%%%%%%%%%%%%%%%%%%%%%

% Use the following line _only_ if you're still using LaTeX 2.09.
%\documentstyle[icml2015,epsf,natbib]{article}
% If you rely on Latex2e packages, like most moden people use this:
\documentclass{article}

% use Times
\usepackage{times}
\usepackage{booktabs}
% For figures
\usepackage{graphicx} % more modern
%\usepackage{epsfig} % less modern
\usepackage{subfigure} 

% For citations
\usepackage{natbib}

% For algorithms
\usepackage{algorithm}
\usepackage{algorithmic}

% As of 2011, we use the hyperref package to produce hyperlinks in the
% resulting PDF.  If this breaks your system, please commend out the
% following usepackage line and replace \usepackage{icml2015} with
% \usepackage[nohyperref]{icml2015} above.
\usepackage{hyperref}

% Packages hyperref and algorithmic misbehave sometimes.  We can fix
% this with the following command.
\newcommand{\theHalgorithm}{\arabic{algorithm}}

% Employ the following version of the ``usepackage'' statement for
% submitting the draft version of the paper for review.  This will set
% the note in the first column to ``Under review.  Do not distribute.''


\usepackage{amsmath}	% required for `\align' (yatex added)
\usepackage{amsfonts}
\usepackage{wrapfig}
\usepackage{amssymb}
\usepackage{amsthm}
\usepackage{cuted}
% Employ this version of the ``usepackage'' statement after the paper has
% been accepted, when creating the final version.  This will set the
% note in the first column to ``Proceedings of the...''
%\usepackage[accepted]{icml2015}
\usepackage[arxiv]{icml2015} 

\input{mathdef}

\usepackage{xr}
\externaldocument{example_paper}
\onecolumn
\begin{document}
\input{supplementary_contents}
\end{document}
